# Supplementary material for: Collaboration Equilibrium in Federated Learning
Source: arXiv:2108.07926 source file (2022-06-02)
Supplement: Supplementary file 1 [file supp.pdf]

## A Algorithm

---

### Algorithm 1: Achieving collaboration equilibrium

---

**Input:**  $N$  institutions  $\mathbf{I} = \{I^i\}_{i=1}^N$  seeking collaborating with others  
Set original client set  $C \leftarrow \mathbf{I}$ ;  
Set collaboration strategy  $S \leftarrow \emptyset$ ;  
**while**  $C \neq \emptyset$  **do**  
    **forall** client  $I^i \in C$  **do**  
        └ Determine the OCS of  $I^i$  by SPO;  
    Construct the benefit graph  $BG(C)$ ;  
    Search for all strongly connected components  $\{C^1, C^2, \dots, C^k\}$  of  $BG(C)$  using **Tarjan** algorithm;  
    **forall**  $i = 1, 2, 3, \dots, k$  **do**  
        **if**  $C^i$  is stable coalition **then**  
            └  $C \leftarrow C \setminus C^i$ ;  
            └  $S \leftarrow S \cup \{C^i\}$ ;  
**Output:** collaboration strategy  $S$

---

When Assumption 1 holds, from Corollary 1 proposed in the main text, the framework for obtaining a collaboration strategy which leads to a CE is simplified as in Algorithm 2.

---

### Algorithm 2: Achieving collaboration equilibrium under Assumption 1

---

**Input:**  $N$  institutions  $\mathbf{I} = \{I^i\}_{i=1}^N$  seeking collaborating with others  
Set original client set  $C \leftarrow \mathbf{I}$ ;  
Set collaboration strategy  $S \leftarrow \emptyset$ ;  
**forall** client  $I^i \in C$  **do**  
    └ Determine the OCS of  $I^i$  by SPO;  
Construct the benefit graph  $BG(C)$ ;  
Search for all strongly connected components  $S = \{C^1, C^2, \dots, C^k\}$  of  $BG(C)$  using **Tarjan** algorithm;  
**Output:** collaboration strategy  $S$

---

## B Proofs of all Theoretical Results

### B.1 Proof of Theorem 1

**Theorem 1.** *Given a client set  $\mathbf{I}$  and its  $BG(\mathbf{I})$ , the stable coalitions are strongly connected components of  $BG(\mathbf{I})$ .*

**Definition 1** (Strongly Connected Component [1]). *A subgraph  $G'$  is a strongly connected component of a given directed graph  $G$  if it satisfies: 1) It is strongly connected, which means that there is a path in each direction between each pair of vertices in  $G'$ ; 2) It is maximal, which means no additional vertices from  $G$  can be included in  $G'$  without breaking the property of being strongly connected.*

To prove Theorem 1, we firstly prove that the benefit graph of a stable coalition is strongly connected shown in Lemma 1.

**Lemma 1.** *For a given client set  $\mathbf{I}$ , the benefit graph  $BG(C^s)$  of each stable coalition  $C^s$  is strongly connected, which means that there is a path in each direction between each pair of vertices in  $BG(C^s)$ .*

*Proof.* We will prove the Lemma 1 by contradiction. Suppose there exists a pair of vertices  $I^1, I^2 \in BG(C^s)$  such that there is no path from  $I^1$  to  $I^2$ , which is denoted as  $\nexists p$ , s.t.,  $I^1 \rightarrow I^2$  for expressive

clearly. We split  $C^s$  into two sub-coalitions  $C'$  and  $C^s \setminus C'$  depending on whether the clients have paths to  $I^2$ . The clients in  $C'$  have no path to  $I^2$ , and the clients in  $C^s \setminus C'$  have paths to  $I^2$ .

$$\begin{aligned} \forall I^i \in C', \nexists p, \text{ s.t., } I^i \rightarrow I^2 \\ \forall I^i \in C^s \setminus C', \exists p, \text{ s.t., } I^i \rightarrow I^2. \end{aligned} \quad (1)$$

Obviously,  $C'$  and  $C^s \setminus C'$  are not empty because  $I^1 \in C'$  and  $I^2 \in C^s \setminus C'$ . From Eq.(5) in the main text in the Definition of *stable coalition*, each client  $I^i \in C^s$  achieves its maximal utility by collaborating with others in  $C^s$  which means that

$$\forall I^i \in C^s, \forall I^j \in C_I^{opt}(I^i), I^j \in C^s. \quad (2)$$

From the Definition of *Optimal Collaborator Set* (OCS), each client  $I^i$  in the OCS of  $I^2$  has an edge from  $I^i$  to  $I^2$ ,

$$\forall I^i \in C_I^{opt}(I^2), \exists p, \text{ s.t., } I^i \rightarrow I^2, \quad (3)$$

Therefore,  $I^2$  can achieve its maximal utility in  $C^s \setminus C'$  because each client  $I^i \in C_I^{opt}(I^2)$  is in  $C^s \setminus C'$ . Moreover, we can prove that  $I^i \in C_I^{opt}(I^2)$  achieves its maximal utility in  $C^s \setminus C'$  because each client  $I^i \in C_I^{opt}(I^2)$  and its corresponding OCS are in  $C^s \setminus C'$ ,

$$\forall I^i \in C_I^{opt}(I^2), \forall I^j \in C_i^{opt}(I^i), \exists p, I^j \rightarrow I^i, \quad (4a)$$

$$\forall I^i \in C_I^{opt}(I^2), \exists p, \text{ s.t., } I^i \rightarrow I^2, \quad (4b)$$

$$\Rightarrow \forall I^i \in C_I^{opt}(I^2), \forall I^j \in C_i^{opt}(I^i), \exists p, I^j \rightarrow I^i \rightarrow I^2 \quad (4c)$$

From Eq.(4), the clients in the OCS of  $I^i \in C_I^{opt}(I^2)$  are in  $C^s \setminus C'$  and  $I^i$  can achieve its optimal utility. Based on the same analysis, for each client  $I^i \in C^s \setminus C'$ , each client  $I^j$  in its OCS  $I^j \in C_i^{opt}(I^i)$  has a path to  $I^2$ . So we have the conclusion that all clients in  $C^s \setminus C'$  achieves its optimal utility by collaborating with others in  $C^s \setminus C'$ . However, this contradicts Eq.(6) in the main text in the Definition of *stable coalition*. Therefore, we prove that the benefit graph  $BG(C^s)$  of each stable coalition  $C^s$  is strongly connected as in Lemma 1.  $\square$

From Lemma 1, the  $BG(C^s)$  is strongly connected, then we will prove that  $BG(C^s)$  is a strongly connected component of  $BG(I)$  by pointing out that  $BG(C^s)$  is maximal which means that no additional vertices from  $I$  can be included in  $BG(C^s)$  without breaking the property of being strongly connected.

*Proof.* We will prove that  $BG(C^s)$  is maximal by contradiction. Suppose there is another client  $I^0 \in I \setminus C^s$  which can be added in  $BG(C^s)$  without breaking the property of being strongly connected. Therefore, there exists  $I^i \in C^s$  which has an edge from  $I^0$  to  $I^i$ . This means that  $I^0$  is one of the necessary collaborators of  $I^i$  ( $I^0 \in C_I^{opt}(I^i)$ ) and  $I^0$  cannot achieve its optimal utility in  $C^s$  without collaborating with  $I^0$ . However, this contradicts Eq.(5) in the main text in the Definition of *stable coalition* that all clients in  $C^s$  can achieve its optimal utility by collaborating with others in  $C^s$ . Therefore, we prove that  $BG(C^s)$  is a strongly connected component as stated in Theorem 1.  $\square$

## B.2 Proof of Theorem 2

**Theorem 2.** *The collaboration strategy  $S = \{C^0, C^1, \dots, C^k\}$  obtained by our proposed method achieves collaboration equilibrium.*

*Proof.* **1. All coalitions in  $S = \{C^0, C^1, \dots, C^k\}$  satisfies Inner Agreement as in Axiom 1.**

As each coalition  $C^i \in S$  is a stable coalition, from Eq.(6) of the Definition of *stable coalition*, we have

$$\forall C^i \in S, \forall C' \subsetneq C^i, \exists I^i \in C', \text{ s.t., } U_{max}(I^i, C') < U_{max}(I^i, C^i). \quad (5)$$

Then Eq.(5) is the definition of *Inner Agreement* in Eq.(3) in the main text. Therefore, we prove that all collaboration coalitions in  $S$  satisfy inner agreement.

## 2. The collaboration strategy $S$ satisfies Outer Agreement as in Axiom 2.

We will prove it by contradiction. Suppose there exists a new nonempty coalition  $C' = \{I^{i^0}, I^{i^1}, \dots, I^{i^k}\} \notin S$  which satisfies

$$\forall I^i \in C', U_{max}(I^i, C') > U_{max}(I^i, C^j) \ (I^i \in C^j \in S). \quad (6)$$

Suppose that  $C^0$  denotes the coalition in the first iteration. Then  $\forall I^i \in C^0$ ,  $I^i$  achieves its maximal utility in the client set  $I$  and cannot increase its model utility further. So we have

$$\forall I^i \in C', I^i \notin C^0. \quad (7)$$

The clients in the coalition  $C^0 \in S$  identified in the first iteration have no interest to collabotatate with others and will be removed. Suppose  $C^1$  denotes the coalition in the first iteration.  $\forall I^i \in C^1$ ,  $I^i$  achieves its maximal utility in the client set  $I \setminus C^0$  and cannot increase its model utility further. So we have

$$\forall I^i \in C', I^i \notin C^1. \quad (8)$$

Then  $C^1$  will be removed and we have  $\forall I^i \in C', I^i \notin I^2..$  Based on the same analysis, we finally have

$$\begin{aligned} \forall I^i \in C', \forall C^j \in S, I^i \notin C^j, \\ \Rightarrow C' = \emptyset. \end{aligned} \quad (9)$$

Therefore, we prove that there is no nonempty  $C'$  satisfying Eq.(6) and  $S$  satisfies Outer Agreement.  $\square$

## B.3 Proof of Corollary 1

**Assumption 1.** *The benefit graph of a subset  $C \subset I$  ( $BG(C)$ ) is the subgraph of the  $BG(I)$ .*

**Corollary.** *When Assumption 1 holds, the strongly connected components of  $BG(I)$  leads to a collaboration equilibrium.*

Firstly, we prove that all strongly connected components are disjoint as in Lemma 2.

**Lemma 2.** *Given a directed graph  $G$  and all its strongly connected components  $\{C^0, \dots, C^k\}$ , each pair of its strongly connected components  $C^i$  and  $C^j$  satisfies  $C^i \cap C^j = \emptyset$ .*

*Proof.* We will prove it by contradiction. Suppose there exists a pair of the strongly connected components which satisfies  $I^0 \in (C^i \cap C^j)$  and  $C = C^i \cup C^j$ . For each pair of vertices  $I^i, I^j$ , we have

$$\begin{aligned} \exists p, I^i \rightarrow I^0 \rightarrow I^j, \\ \exists p, I^j \rightarrow I^0 \rightarrow I^i. \end{aligned} \quad (10)$$

From Eq.(10),  $C$  is strongly connected which conflicts the definition of strongly connected components that each strongly connected component is maximal. Therefore, we prove that  $C^i \cap C^j = \emptyset$ .  $\square$

Theorem 2 states that the collaboration coalitions identified iteratively leads to a *collaboration equilibrium*. To prove the Corollary B.3, we will demonstrate that the collaboration coalitions identified iteratively are all strongly connected components of  $BG(I)$  when Assumption 1 holds.

*Proof.* Suppose the coalitions strategy  $S = \{C^0, C^1, \dots, C^k\}$  is determined iteratively and  $C^i$  is identified in the  $i$ -th iteration. From Theorem 1,  $C^0$  is one of the strongly connected components of  $BG(I)$ . When Assumption 1 holds,  $BG(I \setminus C^0)$  is the subgraph of  $BG(I)$ . This means that any

edge in  $BG(I \setminus C^0)$  is also the edge in  $BG(I)$  and vice versa.  $C^1$  is a stable coalition which is one of the strongly connected componts of  $BG(I \setminus C^0)$ . Therefore,  $BG(C^1)$  is strongly connected in  $BG(I)$ . Suppose  $BG(C^1)$  is not a strongly connected component of  $BG(I)$  and there exists an additional client  $I^i$  which can be added in  $C^1$  without breaking the strongly connected property. From Lemma 2,  $I^i$  cannot be from another strongly connected component, so we have

$$I^i \notin C^0. \quad (11)$$

If  $I^i$  is from  $I \setminus (C^0 \cup C^1)$  and can be added into  $C^1$  without breaking the strongly connected property,  $C^1$  is not a strongly connected component of  $I \setminus C^0$ . So we have

$$I^i \notin I \setminus (C^0 \cup C^1). \quad (12)$$

From Eq.(11) and Eq.(12), there is no additional  $I^i$  which can be added in  $C^1$  without breaking the strongly connected property. So  $C^1$  is a strongly connected component of  $BG(I)$ . For the same analysis, we can prove that  $\forall C^i \in S$ ,  $C^i$  is a strongly connected component of  $BG(I)$  when Assumption 1 holds. Therefore, we prove that the strongly connected components of  $BG(I)$  are the stable coalitions identified iteratively as in Algorithm 1 and these strongly connected components lead to a CE.  $\square$

#### B.4 Proof of Proposition 1

**Definition 2** (Pareto Solution and Pareto Front). *We consider  $n$  objectives corresponding to  $n$  clients:  $l_i : \mathbb{R}^n \rightarrow \mathbb{R}_+, i = \{1, 2, \dots, n\}$ . Given a learned hypothesis  $h$ , suppose the loss vector  $\mathbf{l}(h) = [l_1, l_2, \dots, l_n]$  represents the utility loss on  $n$  clients with hypothesis  $h \in \mathcal{H}$ , we say  $h$  is a Pareto Solution if there is no hypothesis  $h'$  that dominates  $h$ :  $h' \prec h$ , i.e.,*

$$\nexists h' \in \mathcal{H}, \text{ s.t. } \forall i : l_i(h') \leq l_i(h) \text{ and } \exists j : l_j(h') < l_j(h). \quad (13)$$

*In a collaboration network with  $N$  clients  $\{I^i\}_{i=1}^N$ , as each client has its own learning task which can be formulated as a specific objective, we use  $P(\{I^1, I^2, \dots, I^N\})$  to represent the Pareto Front (PF) of the client set  $\{I^i\}_{i=1}^N$  formed by all Pareto hypothesis.*

**Proposition 1** (Pareto Front Embedding Property). *Suppose  $\mathbf{l}^* = [l_i(h^*)], i \in C'$  and  $\mathbf{l}^* = [l_i(h^*)], i \in C$  are the loss vectors achieved by the PFs  $P(C')$  and  $P(C)$  where  $C' \subset C$ , then*

$$\forall h^* \in P(C'), \exists h^* \in P(C), \text{ s.t. }, l_i(h^*) = l_i(h^*) \forall i \in C'. \quad (14)$$

*Proof.* For any hypothesis  $h^* \in P(C')$ ,  $h^*$  satisfies

$$\nexists h' \in \mathcal{H}, \text{ s.t. } \forall i \in C' : l_i(h') \leq l_i(h^*) \text{ and } \exists j : l_j(h') < l_j(h^*). \quad (15)$$

1) If  $h^* \in P(C)$  which satisfies

$$\nexists h' \in \mathcal{H}, \text{ s.t. } \forall i \in C : l_i(h') \leq l_i(h) \text{ and } \exists j : l_j(h') < l_j(h), \quad (16)$$

then we let  $h^* = h^*$  in Eq.(14) so Eq.(14) holds;

2) if  $h^* \notin P(C)$ , there exists  $h' \in P(C)$  which satisfies

$$\forall i \in C : l_i(h') \leq l_i(h^*) \text{ and } \exists j : l_j(h') < l_j(h^*), \quad (17)$$

combining Eq.(15), we have

$$\forall i \in C' : l_i(h') = l_i(h^*) \text{ and } \exists j \in C \setminus C' : l_j(h') < l_j(h^*). \quad (18)$$

then we let  $h^* = h'$  in Eq.(14) so Eq.(14) holds.  $\square$

## C Implementation

In this section, firstly we will introduce how to learn the Pareto Front of all objectives corresponding to all clients. Then, we will describe how to determine the optimal collaborator set for each client.

### C.1 Learning the Pareto Front

Multi-objective optimization (MOO) problems have a set of optimal solutions, and these optimal solutions form the Pareto front, where each point on the front represents a different trade-off between possibly conflicting objectives. We construct a personalized model for each client which we call target network and it has the same architecture as the baselines. To determine the parameters of the target network of each client, in our experiments, we learn the entire Pareto Front simultaneously using a hypernetwork which receives as input a direction vector  $d$  and returns all parameters of the target network. The input direction vector is  $N$ -dimension  $d$  which is sampled from the convex hull  $\mathcal{D}$ ,

$$\mathcal{D} = \left\{ d, |\forall i, 1 \leq i \leq N, d^i \geq 0, \text{ and } \sum_{i=1}^N d^i = 1 \right\}. \quad (19)$$

Specifically, we construct the hypernetwork following in the architecture introduced in [2]. By a  $n$ -layer ( $n \leq 3$ ) MLP network with the activation function ReLU, we inference the parameters of the target network. Then the obtained parameters will be assigned to the target network. We evaluate the performance of the parameters on the training set and the gradient information will be returned for updating the hypernetwork.

### C.2 Identifying the Optimal Collaborator Set

From the statement above, we train a hypernetwork  $HN$  for learning the whole Pareto front.  $HN$  bridges the mapping from the direction vector  $d$  to the corresponding model parameters of the target network. To obtain the optimal parameters of the target network which achieves the minimal value loss of the target objective on the validation set, we optimize the direction vector  $d$  by gradient descent. Specifically, given an initial direction  $d_0$ , we firstly obtain the parameters of the target network using the learned hypernetwork  $HN(d_0)$ . Similarly as training the hypernetwork, the obtained parameters will be assigned to the target network. Then we evaluate the performance of the generated parameters on the validation set and compute the gradient of the input direction  $d_0$ . Then the gradient information will be used for updating the direction vector  $d$  iteratively until convergence.

$$\begin{aligned} d_{i+1} &= d_i - \nabla_{d_i} l^* \\ d_{i+1} &\leftarrow \text{Clip}(d_{i+1}) \\ d_{i+1} &\leftarrow \text{Normalization}(d_{i+1}), \end{aligned} \quad (20)$$

where  $\text{Clip}(d_{i+1})$  means that we clip each values  $d_{i+1}^j \in d_{i+1}$  to satisfy  $\epsilon_0 \leq d_{i+1}^j \leq 1$  and  $\text{Normalization}(d_{i+1})$  means that we normalize  $d_{i+1}$  as follows,

$$\forall j (1 \leq j \leq N), d_{i+1}^j = \frac{d_{i+1}^j}{\sum_{j=1}^N d_{i+1}^j}. \quad (21)$$

Finally, we reach the optimal direction  $d^*$  and its corresponding Pareto model  $M^*$ .

For each client, we determine the optimal collaborator set by the optimal direction  $d^*$  and the loss value of all objectives  $\mathbf{l} = [l_1(M^*), l_2(M^*), \dots, l_N(M^*)]$ . From the Pareto Front Embedded property described in Proposition 1, an ideal direction  $d^*$  is a sparse vector in which the indexes of the non-zero values in  $d^*$  are the necessary collaborators for the target client. In our experiments,  $d^*$  usually is not a sparse vector but there are values in  $d^*$  which are significantly small. Therefore, we set a threshold  $\epsilon$  for  $d^*$  to identify which clients are necessary/unnecessary.

## D Experimental Details

### D.1 Synthetic data experiments

The synthetic data generation process is illustrated in the main text. In this experiment, we construct the hypernetwork using 1-layer hidden MLP for generating the target network parameters and the target network is a 1-layer MLP. The experiments have two settings, 1) 2000 training samples and  $\rho = 0.1$ ; 2) 20000 training samples and  $\rho = 1.0$ .

We plot the direction vector  $d = [d^0, d^1, d^2, d^3, d^4, d^5]$  varies in each iteration as we learn a personalized model for  $I^0$ . When  $n = 2000, \rho = 0.1$  and the target client is  $I^0$ , from Figure 1(a),  $\{d^3, d^4, d^5\}$  decrease until reach the minimum and  $\{d^0, d^1, d^2\}$  increase in each iteration. As  $\rho \neq 0$ , the data in  $I^1$  ( $I^2$ ) and  $I^0$  does not satisfy i.i.d, so  $d^0$  is slightly larger than  $d^1$  and  $d^2$ . This means that the optimal personalized model of  $I^0$  is on  $PF(I^0, I^1, I^2)$  and the OCS of  $I^0$  is  $\{d^0, d^1, d^2\}$ . When  $n = 20000, \rho = 1.0$  and the target client is  $I^0$ , from Figure 1(b),  $\{d^1, d^2, d^3, d^4, d^5\}$  decrease and reach the minimum and  $d^0$  increases in each iteration. This means that the optimal personalized model of  $I^0$  is on  $PF(I^0)$  and the OCS of  $I^0$  is  $\{d^0\}$ .

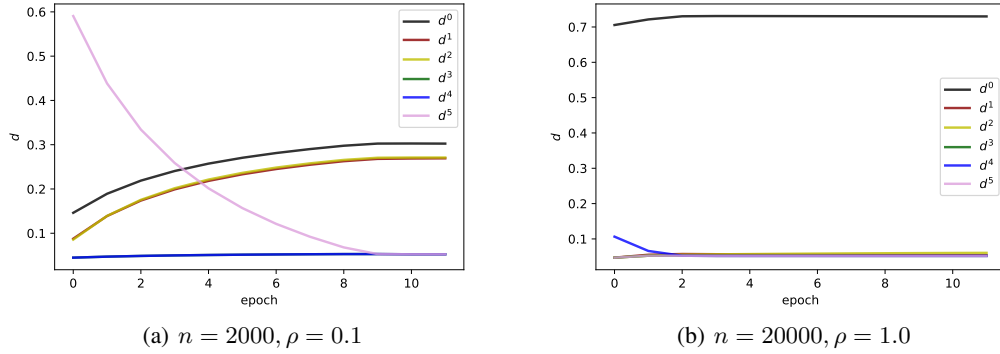

Figure 1:  $d = [d^0, d^1, d^2, d^3, d^4, d^5]$  varies in each iteration where  $d^i$  corresponds to the clients  $I^i$ .

After identifying all coalitions, all clients will re-learn a personalized model by collaborating with other clients in its coalition.

### D.2 UCI Adult data experiments

UCI Adult is a public dataset [3] which is split as training set and test set. We follow the dataset preprocessing procedure as in [4, 5] and split the data into two clients PhD client and Non-PhD client. In this experiment, we construct the hypernetwork using 1-layer hidden MLP. The target network is a Logistic Regression model as in [4, 5]. We split 83% training data for learning the PF and the remaining 17% training data for determining the optimal direction vector  $d$ . All hyper parameters are determined by the performance on the validation data set.

### D.3 CIFAR10 data experiments

CIFAR10 is a public dataset [6] which contains 50000 images for training and 10000 images for testing. In our experiments, we following the setting in [7]. We split the data into 10 clients and simulate non-i.i.d environment by randomly assigning two classes to each client among ten total classes. All training data will be divided into training set (83%) and validation set (17%). We construct the hypernetwork using 3-layer hidden MLP for generating the parameters of the target network and the target network is constructed following the work [8]. All baselines share the same target network structure for each client. To determine the hyper parameters (e.g., learning rate), we evaluate the performance of different hyper parameter combination on the validation set and choose the hyper parameter combination which achieves the optimal accuracy on the validation data set.

## D.4 eICU data experiments

**eICU Data Asset** eICU dataset [9] is a dataset for which permission is required. We followed the procedure on the website <https://eicu-crd.mit.edu> and got the approval to the dataset. In this experiment, we follow the data preprocessing as in [10] and select 10 hospitals for collaboration as introduced in the main text. As all hospitals own relatively insufficient patient data samples ( $100 \leq n \leq 1300$ ), dividing the data into training set and test set in different ways may lead to different CE. We construct the hypernetwork by a 1-layer MLP for training the Pareto Front of all objectives. The target network is an ANN model following the work in [10]. We determine the hyper parameters by evaluating the different hyper parameter combinations on the validation set.

## D.5 Training Resources

We run our experiments on a local Linux server which has two physical CPU chips (Inter(R) Xeon(R) CPU E5-2640 v4 @ 2.40GHz) and 32 logical kernels. We use Pytorch framework to implement our model and train all models on GeForce RTX 2080 Ti GPUs.

## E Discussion

In this work, we study the collaborative learning problem and propose the core goal that the collaboration strategy achieves *collaborative equilibrium* (CE). Achieving collaboration equilibrium needs to identify the necessary/unnecessary collaborators for each client. In theory, it is a combinatorial optimization problem with exponential complexity. There are plenty works on addressing combinatorial optimization problem by reinforcement learning [11]. However, mostly it's hard to obtain stable results using reinforcement learning methods on this problem. We propose to identify the necessary collaborators according to the geometric location of the optimal models which avoids solving this combinatorial optimization problem directly. In theory, there are  $B_N$  collaboration strategies. We propose an iterative method for identifying all collaboration coalitions in polynomial complexity. In order to further reduce complexity, we propose Assumption 1 that all strongly connected components lead to a CE. As our framework quantifies the benefit of each client in a collaborative network, for the impact of our work on the society, some big clients may no longer collaborate with small clients without any charge.

## References

- [1] Robert Tarjan. Depth-first search and linear graph algorithms. *SIAM journal on computing*, 1(2):146–160, 1972.
- [2] Aviv Navon, Aviv Shamsian, Gal Chechik, and Ethan Fetaya. Learning the pareto front with hypernetworks. *arXiv preprint arXiv:2010.04104*, 2020.
- [3] Ron Kohavi. Scaling up the accuracy of naive-bayes classifiers: A decision-tree hybrid. In *Kdd*, volume 96, pages 202–207, 1996.
- [4] Tian Li, Maziar Sanjabi, Ahmad Beirami, and Virginia Smith. Fair resource allocation in federated learning. *arXiv preprint arXiv:1905.10497*, 2019.
- [5] Mehryar Mohri, Gary Sivek, and Ananda Theertha Suresh. Agnostic federated learning. In *International Conference on Machine Learning*, pages 4615–4625. PMLR, 2019.
- [6] Yann LeCun, Léon Bottou, Yoshua Bengio, and Patrick Haffner. Gradient-based learning applied to document recognition. *Proceedings of the IEEE*, 86(11):2278–2324, 1998.
- [7] H Brendan McMahan, Eider Moore, Daniel Ramage, and Blaise Agüera y Arcas. Federated learning of deep networks using model averaging. *arXiv preprint arXiv:1602.05629*, 2016.
- [8] Aviv Shamsian, Aviv Navon, Ethan Fetaya, and Gal Chechik. Personalized federated learning using hypernetworks. *arXiv preprint arXiv:2103.04628*, 2021.
- [9] Tom J Pollard, Alistair EW Johnson, Jesse D Raffa, Leo A Celi, Roger G Mark, and Omar Badawi. The eicu collaborative research database, a freely available multi-center database for critical care research. *Scientific data*, 5(1):1–13, 2018.

- [10] Seyedmostafa Sheikhalishahi, Vevake Balaraman, and Venet Osmani. Benchmarking machine learning models on eicu critical care dataset. *arXiv preprint arXiv:1910.00964*, 2019.
- [11] Nina Mazyavkina, Sergey Sviridov, Sergei Ivanov, and Evgeny Burnaev. Reinforcement learning for combinatorial optimization: A survey. *Computers & Operations Research*, page 105400, 2021.
